# Supplementary material for: CommonCanvas: An Open Diffusion Model Trained with Creative-Commons Images
Source: arXiv:2310.16825 source file (2023-10-25)
Supplement: Supplementary file 1 [file 99-scratch.tex]

\section{Project Plan}
\begin{enumerate}
    \item Target Date: \textbf{ICLR: Sept 28, 2023} \ 
    Backup Deadlines: \textbf{CVPR: November 11, 2022/ICCV Mar 2024} 
    \item \textbf{Goals}:
    \begin{enumerate}
        \item Publish ICLR / CVPR Paper
        \item Publish high res YFCC100M Dataset on Hugging Face
        \item Publish SD2/SDXL trained on YFCC100M on Hugging Face
        \item Publish SD2/SDXL trained on Openverse on Hugging Face (Phase 2)
        \begin{enumerate}
            \item Do coordinated / marketing + press release whenever we do this with Openverse + HF
        \end{enumerate}
        \item Publish MosaicML BlogPost \textbf{(Phase 1 + 2)}
    \end{enumerate}

    \item Two phases:
    \begin{enumerate}
        \item \textbf{Phase 1}: BoB. Release a V0 diffusion model
        \begin{enumerate}
            \item Architecture: Either SD2 or SDXL
            \item 2 Models:
            \begin{enumerate}
                \item YFCC100M CC-0/CC-Commerical
                \item YFCC100m 100M run
            \end{enumerate}
            \begin{enumerate}
                \item If we do SDXL, do a high res version of it 1024x1024 
            \end{enumerate}
            \item SDXL cost estimate breakdown (batch size 2048 on 32 H100s):
            \begin{enumerate}
                \item Stage 1: 256x256 for 600K iterations $\rightarrow$ $\sim$ 3000 H100 hours
                \item Stage 2: 512x512 for 200K iterations $\rightarrow$ $\sim$ 3000 H100 hours
                \item Stage 3: 1024x1024 for 200K iterations $\rightarrow$ $\sim$ 14500 H100 hours (note: 200K here is just a guess, SDXL paper doesn't mention how long they train at this res)
                \item Stage X: We have a lot of 4K images, can we use them? Would be 116000 H100 hours
                \item Also note, these throughputs were estimated with a single text encoder (like SD2) and without conditioning but I don't expect adding those (if we choose to) would make it that much more expensive
                \item this is also for the base SDXL (without extra refiner network). I do expect adding the refiner network would make it more expensive but not sure by how much (no refiner training details in paper)
            \end{enumerate}
        \end{enumerate}
        \item \textbf{Phase 2}: Release Openverse / (V1/V2) version of the model
        \begin{enumerate}

            \item Architecture: Latent Diffusion with a DIT or other improvements + 2X speed, would be the same as the basic training runs of YFCC100M. Could either be done as an improvement to the ICLR paper or a CVPR submission. Likely heavily inspired by SimpleDiffusion. (Scale noise schedule and architecture in a similar way to the paper). 
            \item Dataset : Full Openverse Dataset (700 million images)
             \item Release Openverse Dataset + Openverse Model
            \item Cost Breakdown:
            \begin{enumerate}
                \item Same / 50\% Less than Phase 1. Switching to a VIT backend will drop the cost by 50\%. Potentially fewer experiments needed. Can be rolled into ICLR papers thanks to the long rebuttal time.
            \end{enumerate}
        \end{enumerate}
            
    \end{enumerate}
    \item Experiment Must Haves:
    \begin{enumerate}
        \item Will 200k iterations be good enough for 512x512 phase 2 training of BoB? (5X training cost)
        \item Sweep over dataset size (partially done need to expand) Will use LAION for this (Consider doing on this synthetic caption instead) (256 resolution 256 GPU days H100)~\ref{fig:data-variance}] (10x training cost)
        \item Sweep over model size (to emphasize the model is too small) (256 GPU day H100). Also demonstrate mathematically that's it's probably too small, by compression (4x training cost)
    \end{enumerate}
    Nice to have 
    \begin{enumerate}
        \item V-prediction experiments. Can we get away without noise offset by using v-prediction?
        \item Do we need to scale the data additionally?
        \item Can we leverage more images without captions? What if they are in a different domain? iNaturalist images?
        \item  Scale the Diffusion Model 

    \end{enumerate}
    \item After Training Experiments (no training compute needed)
    \begin{enumerate}
        \item Mickey Mouse Copyright + Pokemon ~\ref{fig:mmouse}
        \item Can we identify Celebrities from MSCeleb? Use off the shelf model trained on them? Shows PII preserving
        \item SD2 Qualitative Comparison
        ~\ref{fig:SD2Compare}
        \item Human Eval / Vibe Checks (just coding / time)
        \item Measure clip-score + diversity of BLIP2 captions vs LAION captions vs YFCC100M Blip2 captions (
    \end{enumerate}
    \item After Data Training
    \begin{enumerate}
        \item Host Data on HuggingFace
        \item Host model on HuggingFace
    \end{enumerate}
\end{enumerate}

Success/Completion Criteria Goals:
\begin{enumerate}
    \item Diffusion Model Released
    \item 
\end{enumerate}

\section{Evaluation}
\begin{itemize}
    \item Local Narrative (Open Images) - CLIP/FID
    \item Celebrity Identification (MS-CELEB-1M) - classifier based
    \item Metrics on Google WIT dataset?
    \item N-GRAM Diversity vs CLIP SCore of captions
    \item Zero Shot - Eval on ImageNet % N-FOLD FID calculation <=> metric / Try on ImageNet? MS-Celeb
    \item CLIP Score + FID + KID + CLIP-FID on COCO2014
    \item Human evaluation on parti prompts
    \item CLIP/FID eval on conceptual captions subsests?
    % \item Find a mascot dataset?
    \item FineTune (Likely Post Rebuttal)
    \begin{enumerate}
        \item Finetune on Anime? Met Art Dataset
        \item MetFaces dataset -> Sg2
        \item INaturalist
        \item Danbooru 
    \end{enumerate}
    
\end{itemize}

\section{Legal Justification}

The legal issues related to the use of copyrighted text and images in training machine learning models are complex and multi-faceted. The primary concerns revolve around the concepts of originality, fixation, transformative nature, direct copying, machine learning as a tool, and the doctrine of fair use. Additionally, the Chaffee Amendment and the Marrakesh Treaty provide specific protections for the use of copyrighted works for accessibility purposes.

Short captions which describe factual contents in an image are not copyrightable. Consequently, even if we presume that training copyrighted text was not a transformative work, all research in Large Language Models (LLMs) would not necessarily have to cease due to the large nature of the text. Further details can be found at \href{https://fairuse.stanford.edu/2003/09/09/copyright_protection_for_short/}{Stanford's Fair Use Project}.
